# Supplementary material for: Predicting the Target Word of Game-playing Conversations using a Low-Rank Dialect Adapter for Decoder Models
Source: arXiv:2409.00358 source file (2025-01-31)
Supplement: Supplementary file 1 [file errors.tex]

\section{en-IN Features}\label{sec:dial_feat}
